# Supplementary material for: Model for Topological Phononics and Phonon Diode
Source: arXiv:1606.08013 source file (2017-08-08)
Supplement: Supplementary file 1 [file suppl.pdf]

# Model for Topological Phononics and Phonon Diode

Yizhou Liu[1,2,3], Yong Xu[1,2,3,*] Shou-Cheng Zhang[4,5], and Wenhui Duan[1,2,5†]
[1]*State Key Laboratory of Low Dimensional Quantum Physics, Department of Physics, Tsinghua University, Beijing 100084, People's Republic of China*
[2]*Collaborative Innovation Center of Quantum Matter, Beijing 100084, People's Republic of China*
[3]*RIKEN Center for Emergent Matter Science (CEMS), Wako, Saitama 351-0198, Japan*
[4]*Department of Physics, McCullough Building, Stanford University, Stanford, California 94305-4045, USA*
[5]*Institute for Advanced Study, Tsinghua University, Beijing 100084, People's Republic of China*

The Supplementary Materials include description of seven parts: (i) the time reversal symmetry (TRS)-breaking terms of a harmonic Lagrangian, (ii) the Schrödinger-like equation of phonons, (iii) an effective Hamiltonian, (iv) molecular dynamics simulations, (v) the phonon diode effect and (vi) the influence of out-of-plane vibrations.

## I. THE TRS-BREAKING TERMS OF A HARMONIC LAGRANGIAN

Generally, there are three possible kinds of quadratic terms that could break TRS in a harmonic Lagrangian, including $\tilde{m}_i\dot{u}_i^2$, $\tilde{D}_{ij}u_iu_j$ and $\eta_{ij}\dot{u}_iu_j$, where $\tilde{m}_i$ and $\tilde{D}_{ij}$ are imaginary, and $\eta_{ij}$ is real. All these terms are odd under the time-reversal operation $\Theta = \sigma_t\mathcal{K}$, where $\sigma_t$ changes $t$ into $-t$ and $\mathcal{K}$ is the complex conjugate. The first two kinds of terms are excluded considering that the Hamiltonian should be Hermitian for ensuring real eigenvalues and probability conservation. For the $\eta_{ij}\dot{u}_iu_j$ term, its symmetric part can be written as the time derivative of $\eta^S_{ij}u_iu_j$, which only contributes a constant into the action $\mathcal{S} = \int_{t_1}^{t_2} L\, dt$ and thus does not affect the equation of motion. Therefore, the only possible TRS-breaking term that is physically allowed in a harmonic Lagrangian is of the form

$$L' = \eta_{ij}\dot{u}_iu_j, \tag{1}$$

where the matrix $\eta$ is real and antisymmetric.

## II. THE SCHRÖDINGER-LIKE EQUATION OF PHONONS

The Hamiltonian of a harmonic lattice is

$$H = \frac{1}{2}(p_i - \eta_{ij}u_j)^2 + \frac{1}{2}D_{ij}u_iu_j, \tag{2}$$

where $p_i = \partial L/\partial u_i = \dot{u}_i + \eta_{ij}u_j$ is the canonical momentum and the Lagrangian $L = L_0 + L'$. Define an extended coordinate-velocity space $(y_1, y_2, ..., y_{2dN}) = (u_1, u_2, ..., u_{dN}, \dot{u}_1, \dot{u}_2, ..., \dot{u}_{dN})$, the Hamiltonian is written as $H = \frac{1}{2}Q_{ij}y_iy_j$, where

$$Q = \begin{pmatrix} D & 0 \\ 0 & I_{dN} \end{pmatrix}. \tag{3}$$

Using the Poisson bracket $\{A, B\} = \sum_i(\frac{\partial A}{\partial u_i}\frac{\partial B}{\partial p_i} - \frac{\partial A}{\partial p_i}\frac{\partial B}{\partial u_i})$, we get $\{y_i, y_j\} = -iR_{ij}$, where

$$R = \begin{pmatrix} 0 & iI_{dN} \\ -iI_{dN} & -2i\eta \end{pmatrix}. \tag{4}$$

$I_{dN}$ represents a $dN \times dN$ identity matrix. The equation of motion $\dot{y}_i = \{y_i, H\}$ is simplified into

$$iR^{-1}\dot{y} = Qy. \tag{5}$$

Assuming $y = \tilde{y}e^{-i\omega t}$, the above equation is changed into a generalized Hermitian eigenvalue problem

$$Q\tilde{y} = \omega R^{-1}\tilde{y}, \tag{6}$$

where both $R$ and $Q$ are Hermitian. $Q$ is semi-positive-definite as required by the structural stability of the system, and thus $Q^{1/2}$ is Hermitian. After making a transformation

$$\psi = Q^{1/2}\tilde{y} = \begin{pmatrix} D^{1/2}u \\ \dot{u} \end{pmatrix}, \tag{7}$$

we get a Schrödinger-like equation of phonons in the real space: $\mathcal{H}\psi = \omega\psi$, where the Hamiltonian is

$$\mathcal{H} = Q^{1/2}RQ^{1/2} = \begin{pmatrix} 0 & iD^{1/2} \\ -iD^{1/2} & -2i\eta \end{pmatrix}. \tag{8}$$

After Fourier transforms we get a Schrödinger-like equation of phonons in the **k**-space: $H_{\mathbf{k}}\psi_{\mathbf{k}} = \omega_{\mathbf{k}}\psi_{\mathbf{k}}$, where

$$H_{\mathbf{k}} = \begin{pmatrix} 0 & iD_{\mathbf{k}}^{1/2} \\ -iD_{\mathbf{k}}^{1/2} & -2i\eta_{\mathbf{k}} \end{pmatrix}, \psi_{\mathbf{k}} = \begin{pmatrix} D_{\mathbf{k}}^{1/2}\mathbf{u}_{\mathbf{k}} \\ \dot{\mathbf{u}}_{\mathbf{k}} \end{pmatrix}. \tag{9}$$

Here $D_{\mathbf{k}}$ is positive-semidefinite as required by the structural stability, and its square root $D_{\mathbf{k}}^{1/2}$ is thus Hermitian, which together with the anti-Hermitian $\eta_{\mathbf{k}}$ gives a Hermitian Hamiltonian $H_{\mathbf{k}}$. The equation has some important features:

(i) The phonon wavefunction $\psi_{\mathbf{k}}$ is defined in the extended coordinate-velocity space, including two subspaces $\psi^1_{\mathbf{k}} = D_{\mathbf{k}}^{1/2}\mathbf{u}_k$ and $\psi^2_{\mathbf{k}} = \dot{\mathbf{u}}_k$. When TRS is preserved ($\eta_{\mathbf{k}} = 0$), the two subspaces are not independent of each other but related by $\psi^2_{\mathbf{k}} = \pm i\psi^1_{\mathbf{k}}$. Thus using either subspace is enough to describe phonons. The situation is similar for electrons. While the two-component spinor wavefunction is required in general, only the one-component wavefunction is necessary for describing spin-degenerate systems.

(ii) The phonon Hamiltonian has $2dN$ eigenvalues, but the system only has $dN$ degrees of freedom. The discrepancy is explained by a "particle-hole" symmetry, $\{H, K\} = 0$ ($K$ is the complex conjugate operator), which guarantees $(\omega_{\mathbf{k}}, \psi_{\mathbf{k}})$ and $(-\omega_{-\mathbf{k}}, \psi^*_{\mathbf{k}})$ appear in pairs.

(iii) Based on the Schrödinger-like equation, all topology-related quantities of phonons can be defined similar as for electrons. For the $n$th band, $\psi_{n\mathbf{k}}$ is the phonon wavefunction, the Berry connection $\mathbf{A}_{n\mathbf{k}} = -i\psi^\dagger_{n\mathbf{k}}\nabla_{\mathbf{k}}\psi_{n\mathbf{k}}$, the Berry curvature $\mathbf{B}_{n\mathbf{k}} = \nabla_{\mathbf{k}} \times \mathbf{A}_{n\mathbf{k}}$, and the Chern number $C_n = \frac{1}{2\pi}\iint_{BZ} d^2\mathbf{k} B_{z,n\mathbf{k}}$. The total Chern number $C$ is the summation over all the Chern numbers of bands below a specified band gap.

(iv) Under inversion symmetry, $\omega_{n\mathbf{k}} = \omega_{n,-\mathbf{k}}$ and $\mathbf{B}_{n\mathbf{k}} = \mathbf{B}_{n,-\mathbf{k}}$. Under TRS, $\omega_{n\mathbf{k}} = \omega_{n,-\mathbf{k}}$, $\mathbf{B}_{n\mathbf{k}} = -\mathbf{B}_{n,-\mathbf{k}}$ and $C \equiv 0$.

A previous work also employed Hamiltonian mechanics to study topological properties of phonons [1]. In contrast, they used a different Hamiltonian equation together with a non-Hermitian Hamiltonian. As a result, the left eigenvector is different from the right one in Ref. 1. The difference does not affect the discussion of the topological invariant Chern number, but will produce qualitatively different wavefunctions and Berry curvatures. As known for electrons, Hermiticity is an essential property of the Schrodinger equation. Hermitian Hamiltonian is required for a proper definition of the wavefunction. In other words, we feel our results are physically more appealing.

## III. AN EFFECTIVE HAMILTONIAN

In this section we derive an effective Hamiltonian for phonons around the Dirac point, based on symmetry analysis. The main symmetry operations of the honeycomb lattice include $C_{3v}$, space inversion $\mathcal{P}$ and time reversal $\Theta$, where $C_{3v}$ can be decomposed into $C_3$ (3-fold rotation about the out-of-plane $z$-axis) and $\sigma_v$ (mirror operation about the in-plane $x$-axis along the armchair direction).

In the Schrödinger-like equation of phonons, the Hamiltonian $H_{\mathbf{k}}$ is related to the dynamic matrix $D_{\mathbf{k}}$ through

$$H_{\mathbf{k}} = -s_y \otimes D^{1/2}_{\mathbf{k}} + (1 - s_z) \otimes (-i\eta_{\mathbf{k}}), \tag{10}$$

where $s_y$ is the Pauli matrix with $s_y = \mp 1$ referring to positive (negative) frequency branch when TRS is preserved ($\eta_{\mathbf{k}} = 0$). Since the positive and negative frequency branches are related by a "particle-hole" symmetry, we can only consider the positive frequency branch $\left|s_y = -1\right\rangle$. We project the Hamiltonian into the subspace of $\left|s_y = -1\right\rangle$ and get a reduced Hamiltonian

$$\tilde{H}_{\mathbf{k}} = \left\langle s_y = -1\right| H_{\mathbf{k}} \left|s_y = -1\right\rangle = D^{1/2}_{\mathbf{k}} - i\eta_{\mathbf{k}}. \tag{11}$$

The reduced Hamiltonian can be used to describe phonons around the Dirac point, when the coupling between positive and negative frequency branches can be neglected. In the following, we will only consider the positive frequency branch and construct an effective Hamiltonian for the reduced Hamiltonian that will be denoted by $H_{\mathbf{k}}$ as well for simplicity.

**An effective Hamiltonian without symmetry breaking**

When both inversion symmetry and TRS are preserved, the longitudinal acoustic (LA) and longitudinal optical (LO) modes form a linear Dirac-like dispersion near the $K$ ($K'$) point. We choose a representation of $(u_{Ax}, u_{Ay}, u_{Bx}, u_{By})^T$, which corresponds to displacements of the $A(B)$ sublattice along the $x(y)$ direction. The eigenvectors of dynamic matrix at the $K$ point are expressed as

$$\begin{aligned} u_A(K) &= \frac{1}{\sqrt{2}}\begin{pmatrix} 1 \\ -i \\ 0 \\ 0 \end{pmatrix}, \\ u_B(K) &= \frac{1}{\sqrt{2}}\begin{pmatrix} 0 \\ 0 \\ 1 \\ i \end{pmatrix}, \end{aligned} \tag{12}$$

where $u_A(K)$ and $u_B(K)$ have non-zero components only on the $A$ and $B$ sites, respectively. The eigenvectors at the $K'$ point are related to those at the $K$ point by TRS:

$$\begin{aligned} u_A(K') &= u_A(K)^* = \frac{1}{\sqrt{2}}\begin{pmatrix} 1 \\ i \\ 0 \\ 0 \end{pmatrix}, \\ u_B(K') &= u_B(K)^* = \frac{1}{\sqrt{2}}\begin{pmatrix} 0 \\ 0 \\ 1 \\ -i \end{pmatrix}. \end{aligned} \tag{13}$$

These four eigenvectors forms a complete basis that will be used in the following.

Define Pauli matrices $\sigma$ and $\tau$ with $\sigma_z = \pm 1$ and $\tau_z = \pm 1$ referring to $A(B)$ sublattice and valley index $K$ ($K'$), respectively. The four basis functions are labelled by index $\sigma_z$ and $\tau_z$. For instance, $u_A(K) = |\sigma_z = 1, \tau_z = 1\rangle$ and $u_B(K') = |\sigma_z = -1, \tau_z = -1\rangle$. Then the symmetry operations are written as

$$\begin{aligned} C_3 &= e^{i\theta\sigma_z\tau_z}, \\ \sigma_v &= \tau_x, \\ \mathcal{P} &= -\sigma_x\tau_x, \\ \Theta &= \tau_x\mathcal{K}, \end{aligned} \tag{14}$$

where $\theta = 2\pi/3$.

For a given symmetry operation $S$, the dynamic matrix $D_{\mathbf{k}}$ is required to satisfy the symmetry condition: $SD_{\mathbf{k}}S^{-1} = D_{S\mathbf{k}}$. Here $\mathbf{k}$ is referenced to $K$ ($K'$) and $D_{\mathbf{k}}$ is expanded around $\mathbf{k} = 0$. Among all the terms of $D_{\mathbf{k}}$ up to the first order of $\mathbf{k}$,

TABLE I: Transformation table showing that terms of Eq. 15 are even ("+") or odd ("−") under symmetry operations $\mathcal{P}$, $\Theta$ and $\sigma_v$.

| | $d_0$ | $d_1$ | $d_2$ | $d_3$ | $d_4$ | $d_5$ | $d_6$ | $d_7$ | $d_8$ | $d_9$ | $d_{10}$ | $d_{11}$ |
|---|---|---|---|---|---|---|---|---|---|---|---|---|
| $\mathcal{P} = -\sigma_x\tau_x$ | + | + | + | − | − | + | + | − | − | − | − | + |
| $\Theta = \tau_x\mathcal{K}$ | + | + | + | − | − | − | − | − | − | + | − | − |
| $\sigma_v = \tau_x$ | + | − | + | + | − | + | − | + | − | + | − | − |

twelve of them are $C_3$-invariant:

$$\begin{aligned} D_{\mathbf{k}} &= d_0 + d_1(\mathbf{k}) + d_2(\mathbf{k}) + d_3(\mathbf{k}) + d_4(\mathbf{k}) \\ &\quad + d_5(\mathbf{k}) + d_6(\mathbf{k}) + d_7(\mathbf{k}) + d_8(\mathbf{k}) \\ &\quad + d_9(\mathbf{k}) + d_{10}(\mathbf{k}) + d_{11}(\mathbf{k}) \\ &= \omega_D^2 + c_1(k_x\tau_z\sigma_x + k_y\sigma_y) + c_2(k_y\tau_z\sigma_x - k_x\sigma_y) \\ &\quad + c_3(k_x\sigma_x + k_y\tau_z\sigma_y) + c_4(k_y\sigma_x - k_x\tau_z\sigma_y) \\ &\quad + c_5(k_x\sigma_z\tau_x + k_y\tau_y) + c_6(k_y\sigma_z\tau_x - k_x\tau_y) \\ &\quad + c_7(k_x\tau_x + k_y\sigma_z\tau_y) + c_8(k_y\tau_x - k_x\sigma_z\tau_y) \\ &\quad + c_9\sigma_z + c_{10}\tau_z + c_{11}\sigma_z\tau_z, \end{aligned} \tag{15}$$

where $\omega_D$ is the phonon frequency of the Dirac point, and $c_i$ ($i = 1, 2, ..., 11$) are constants. These terms are even or odd under symmetry operations $\sigma_v$, $\mathcal{P}$ and $\mathcal{T}$, as summarized in Table I. It is obviously that only the $d_0$ and $d_2(\mathbf{k})$ terms are invariant under all these symmetry operations. Therefore, the effective Hamiltonian without symmetry breaking is written as

$$\begin{aligned} H_0(\mathbf{k}) &= D_{\mathbf{k}}^{1/2} = \sqrt{d_0 + d_2(\mathbf{k})} \\ &\approx \omega_D + \frac{1}{2\omega_D} d_2(\mathbf{k}) \\ &= \omega_D + v_D(k_y\sigma_x - k_x\sigma_y) \end{aligned} \tag{16}$$

where $v_D$ is the group velocity around the Dirac point.

This Hamiltonian describes the linear gapless phonon dispersions at $K$ ($K'$). If terms proportional to $\sigma_z$ and $\sigma_z\tau_z$ are added into the Hamiltonian, a band gap could be opened at the Dirac point. $\sigma_z$ is odd under parity that exchanges the $A$ and $B$ sublattices. $\tau_z$ is odd under both parity and time reversal that exchanges the $K$ and $K'$ valleys. Thus the $\sigma_z$ term breaks inversion symmetry and the $\sigma_z\tau_z$ term breaks TRS.

**The inversion symmetry-breaking mass term**

Inversion symmetry is broken by a nonzero $\delta$, defined as $m_A = m(1-\delta)$ and $m_B = m(1+\delta)$. Compared to the unperturbed case of $m_A = m_B = m$, a perturbation term is added into the dynamic matrix caused by the nonzero $\delta$:

$$D'_{\mathbf{k}} = \omega_D^2 \begin{pmatrix} \delta & 0 & 0 & 0 \\ 0 & \delta & 0 & 0 \\ 0 & 0 & -\delta & 0 \\ 0 & 0 & 0 & -\delta \end{pmatrix} + O(\delta^2). \tag{17}$$

Correspondingly, a perturbation term $H'_I$ is added into the effective Hamiltonian: $H'_I \approx \sqrt{\omega_D^2 + D'_{\mathbf{k}}} - \omega_D \approx D'_{\mathbf{k}}/2\omega_D$. Using the basis of $[u_A(K), u_B(K), u_A(K'), u_B(K')]$, $H'_I$ is expressed as

$$H'_I = \frac{\omega_D\delta}{2} \begin{pmatrix} 1 & 0 & 0 & 0 \\ 0 & -1 & 0 & 0 \\ 0 & 0 & 1 & 0 \\ 0 & 0 & 0 & -1 \end{pmatrix}. \tag{18}$$

We thus have

$$H'_I = \frac{\omega_D\delta}{2}\sigma_z. \tag{19}$$

**The TRS-breaking mass term**

TRS is broken by a nonzero $\eta$. For a two-dimensional lattice with a Coriolis field of out-of-plane angular velocity $\Omega_z$, the matrix form of $\eta$ is given by

$$\eta = \begin{pmatrix} 0 & -\Omega_z & 0 & 0 \\ \Omega_z & 0 & 0 & 0 \\ 0 & 0 & 0 & -\Omega_z \\ 0 & 0 & \Omega_z & 0 \end{pmatrix}. \tag{20}$$

Due to the nonzero $\eta$, a perturbation term $H'_T$ is added into the effective Hamiltonian: $H'_T = -i\eta$. Using the basis of $[u_A(K), u_B(K), u_A(K'), u_B(K')]$, $H'_T$ is expressed as

$$H'_T = \Omega_z \begin{pmatrix} 1 & 0 & 0 & 0 \\ 0 & -1 & 0 & 0 \\ 0 & 0 & -1 & 0 \\ 0 & 0 & 0 & 1 \end{pmatrix}. \tag{21}$$

We thus have

$$H'_T = \Omega_z\sigma_z\tau_z. \tag{22}$$

This term is actually a Haldane-type mass term [2, 3], which gives a phononic analog of the Haldane model. Though sharing the same form, this model differs considerably from the original Haldane model. Specifically, the Haldane model of spinless electrons is proposed by using imaginary next-nearest-neighbor hopping generated through staggered magnetic flux [2], which is difficult to realize experimentally. Furthermore, a vanishing Haldane term would be obtained if only the $p_z$ orbital is considered for spinless electrons in graphene [4]. In contrast, we proposed a phononic analog of the Haldane model by using a TRS-breaking field. Importantly, our Haldane term is not forbidden by local orbital constraints, because our phononic analog of the Haldane model is built with the $p_x \pm ip_y$ orbitals ($l_z = \pm 1$) of in-plane vibrations [see Eqs. (15,16) in the SM], which couple more effectively with the TRS-breaking field than the $p_z$ orbital ($l_z = 0$).

### Chern number of other band gaps

In the our discussion, we mainly focus on properties of the Dirac gap. Actually, the two-fold band degeneracies at the Γ point can be lifted by Coriolis/magnetic field [Fig. 1(d)]. This opens two additional band gaps at the Γ point. Both of them are topologically nontrivial ($C = 1$) when $m_T \neq 0$, insensitive to the parameter $m_I$. The one-way edge states would appear if having a global band gap between the split bands, which is the case for the gap between the two uppermost bands [Fig. 2(b)].

### Berry curvature, Chern number and the one-way edge states

To verify the topological nature, we calculate the Berry curvature $B_{\mathbf{k}}$ and Chern number $C$ of the Dirac gap. When $m_I = m_T = 0$, $B_{\mathbf{k}}$ is zero everywhere except diverging at the degenerate Dirac points. The Berry phase enclosing the Dirac point is $\pi$ ($-\pi$) at $K$ ($K'$). With a small nonzero mass term $m_I$ or $m_T$, $B_{\mathbf{k}}$ displays finite peaks centered at $K$ ($K'$) and is nearly zero elsewhere [Figs. 1(e,f)]. The integration of each peak gives a Berry phase of $\pm\pi$. Berry phases of the two peaks cancel when breaking inversion symmetry ($m_I \neq 0$), giving a trivial gap with $C = 0$; they add when breaking TRS ($m_T \neq 0$), giving a topologically nontrivial gap with $C = 1$.

One prominent feature of the QAH effect of electrons is the existence of gapless one-way (or chiral) edge states immune to disorders [2, 5]. This is a topological property independent of the statistics. The existence of one-way edge states has been confirmed previously for phonons [6–9], but a quantum mechanical study is still missing to prove their robustness to disorders. To demonstrate the feature explicitly, we calculated the phonon band structure for a nanoribbon structure with $m_T = 0.1$ and further performed transport calculations by the generalize nonequilibrium Green's function method to explore disorder effects (Fig. 2). Gapless edge states are clearly visualized within the Dirac gap, which are forward-moving along one edge and backward-moving along the other edge [Fig. 2(b)]. Disorder scattering significantly suppresses transmission of all phonon states except the one-way edge states [Fig. 2(c)]. Our results clearly prove that transport of the one-way edge phonon modes is ballistic and unaffected by disorders due to its unidirectional nature.

## IV. MOLECULAR DYNAMICS SIMULATIONS

In this section, we use molecular dynamics to simulate lattice vibration in a two-dimensional honeycomb lattice composed of the two regions of $C = 0$ and $C = 1$, respectively [Fig.S1(a)]. In contrast to the usual way of choosing the $C = 0$ region as vacuum, we build the topological phase boundary within the material, advantageous for circuit design. This is realized by using a homogeneous TRS-breaking field $m_T$ and locally varying inversion symmetry-breaking parameter $m_I$. Here the two regions are constructed with parameters $m_I = 0, m_T = 0.1$ for $C = 1$ and $m_I = 0.2, m_T = 0.1$ for $C = 0$, and free boundary condition is selected for the outer boundary atoms.

To visualized the edge-state transport, we applied an external driving force $\mathbf{F}(t) = \mathbf{F}_0 e^{-i\omega_D t}$ on an atom close to the boundary, where the Dirac frequency $\omega_D$ is within the bulk gap. As shown in Fig.S1(b-f), the lattice vibration is localized on the boundary, indicating that only boundary modes are excited. Moreover, the vibration can only transport unidirectionally along the boundary. Our results thus demonstrate the existence of one-way edge modes within the bulk gap, as expected from the topological nature of the system.

## V. THE PHONON DIODE EFFECT

### Zero diode effect in two-terminal coherent transport

The phonon diode effect is always zero for two-terminal coherent transport. This result can be understood as follows. Phonon transport through a linear system is described by a scattering matrix $S$. The matrix element $S_{ij}$ characterizes the complex amplitude of an output in the $j$th terminal induced by an input of unity amplitude in the $i$th terminal. $S$ is unitary as required by power conservation. If together with TRS that requires $S^{-1} = S^*$ [10], $S$ would be symmetric, $S_{ij} = S_{ji}$, giving zero diode effect. $S$ is generally not symmetric when TRS is broken. However, for a two-terminal transport system, the unitary condition of $|S_{12}|^2+|S_{11}|^2 = |S_{21}|^2+|S_{11}|^2 = 1$ enforces a direction-independent transmission $|S_{12}|^2 = |S_{21}|^2$ even with broken TRS. Note that the conclusion applies only to a purely coherent system. Nonzero diode effect is possible for a two-terminal transport system if including the phase-breaking effect that can be simulated by attaching probe terminals in the scattering region [11, 12].

### A concept of selective scattering for phonon diode

For generic phonon states, the diode effect can be tuned based on the information of real-space distribution of phonon states (i.e., $\psi_{\mathbf{k},\mu}$, the wave function projected onto the $\mu$-th atom). When TRS is broken, we generally have $|\psi_{\mathbf{k},\mu}|^2 \neq |\psi_{-\mathbf{k},\mu}|^2$. Then for some specific phonon modes, the forward- and backward-moving states ($\psi_{\mathbf{k}}$ and $\psi_{-\mathbf{k}}$) can be separated in real space as schematically shown in Fig. 4(c), which is confirmed by our calculations (data not shown). With such a space-separated feature, it is possible to introduce defects/disorders mainly along the transport path of $\psi_{\mathbf{k}}$. As a result, the state $\psi_{\mathbf{k}}$ will be scattered by the defects/disorders, whereas the opposite-moving state $\psi_{-\mathbf{k}}$ is much less affected. This concept of selective scattering [illustrated in Fig. 4(c)] can be used to enhance the diode effect.

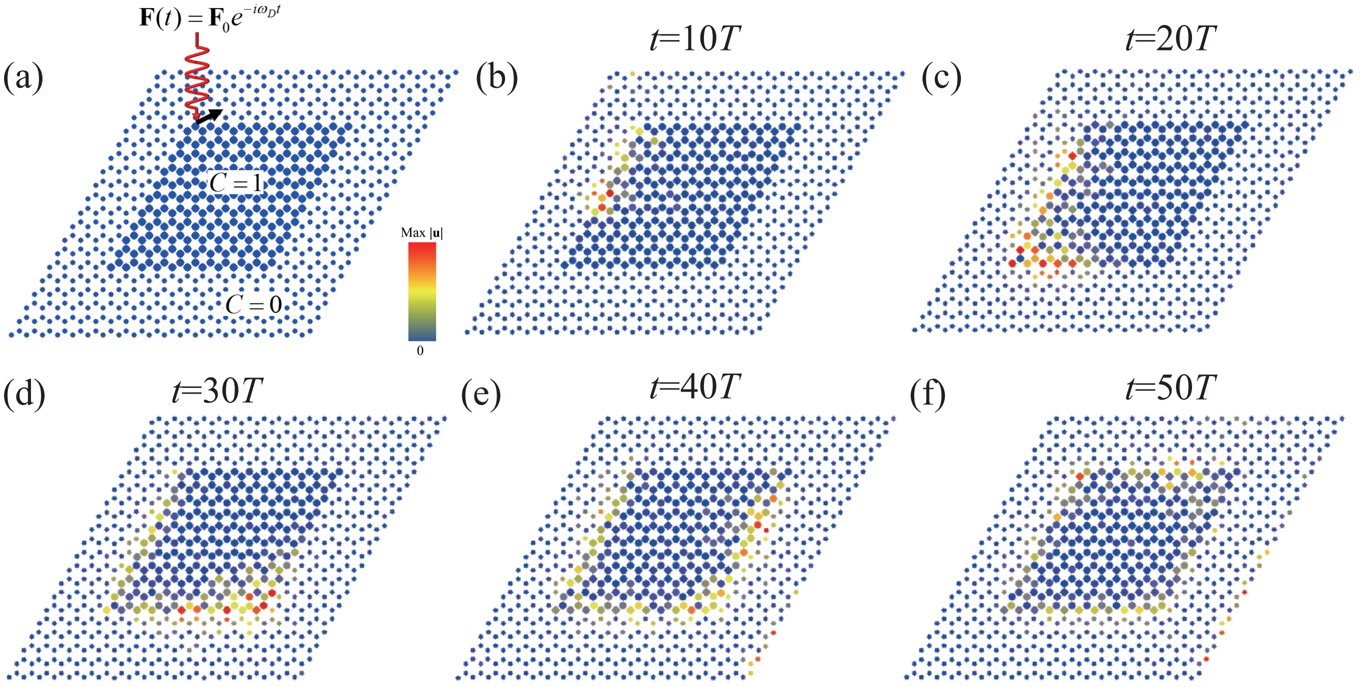


FIG. S1: (a) A two-dimensional honeycomb lattice composed of two regions: $C = 1$ ($m_I = 0, m_T = 0.1$) and $C = 0$ ($m_I = 0.2, m_T = 0.1$), whose atoms are denoted by larger and smaller blue balls, respectively. An external driving force $\boldsymbol{F}(t) = [F_x(t), F_y(t)] = (0.1, 0.1)e^{-i\omega_D t}$ is applied on an atom close to the boundary, where $\omega_D$ is the Dirac frequency. (b)-(f) Snapshots of the displacement distribution at varying time points $t = 10, 20, 30, 40, 50T$, respectively, where $T = 2\pi/\omega_D$. The atoms with the largest (zero) amplitude of displacement are colored red (black) as shown by the color bar in the inset of (b).

## VI. THE INFLUENCE OF OUT-OF-PLANE VIBRATIONS

As shown in Fig.S2, out-of-plane vibrations in a honeycomb lattice introduce two additional phonon bands (one acoustic and one optical), denoted by "ZA" and "ZO", respectively. The two bands cross linearly and form Dirac cones at the $K$ and $K'$ points when both inversion symmetry and TRS are preserved [Fig.S2(a)]. The low-energy physics around the Dirac points is also described by the effective Hamiltonian [Eqs. (5-7)], similar as for in-plane vibrations. Importantly, the effective Hamiltonian is built with the $p_z$ orbital for out-of-plane vibrations in contrast to the $p_x \pm ip_y$ orbitals for in-plane vibrations. When inversion symmetry is broken, band gaps open at the Dirac points for both in-plane and out-of-plane vibrations [Fig.S2(b)]. When TRS is broken by applying a magnetic or Coriolis field along the out-of-plane direction, the "ZA-ZO" Dirac cones keep gapless, while the "LA-LO" Dirac cones become gapped [Fig.S2(c)], demonstrating that the $p_x \pm ip_y$ orbitals ($l_z = \pm 1$) couples more effectively with the TRS-breaking field than the $p_z$ orbital ($l_z = 0$). For the $p_z$ orbital of out-of-plane vibrations, atomic displacements are along the direction of the magnetic or Coriolis field, resulting in a zero Lorentz or Coriolis force and a vanishing Haldane gap in the "ZA-ZO" Dirac cones.

While out-of-plane and in-plane vibrations are decoupled with each other in an atomically flat structure like graphene, they are allowed to hybridize in a buckled structure like silicene, leading to avoided crossings in the phonon dispersion. The hybridization, however, does not break the Dirac cones and typically will not change the topological physics around the Dirac points. Moreover, we notice that the "ZA-ZO" Dirac cones usually overlap with the "TA" and "LA" bands in frequency, which complicates the study of band topology. Such a disadvantage could be avoided for the "LA-LO" Dirac cones. For simplicity, we focused on discussing in-plane vibrations in the main text. But the main conclusions will not be affected if taking out-of-plane vibrations into consideration.


* Electronic address: yongxu@mail.tsinghua.edu.cn

† Electronic address: dwh@phys.tsinghua.edu.cn



[1] L. Zhang, J. Ren, J.-S. Wang, and B. Li, Phys. Rev. Lett. **105**, 225901 (2010).

[2] F. D. M. Haldane, Phys. Rev. Lett. **61**, 2015 (1988).

[3] C. L. Kane and E. J. Mele, Phys. Rev. Lett. **95**, 226801 (2005).

[4] W. J. Elder, E. S. Tok, D. D. Vvedensky, and J. Zhang, arXiv:1306.2520 (2013).

[5] C.-Z. Chang, J. Zhang, X. Feng, J. Shen, Z. Zhang, M. Guo, K. Li, Y. Ou, P. Wei, L.-L. Wang, et al., Science **340**, 167 (2013).

[6] E. Prodan and C. Prodan, Phys. Rev. Lett. **103**, 248101 (2009).

[7] Y.-T. Wang, P.-G. Luan, and S. Zhang, New J. Phys. **17**, 073031 (2015).

[8] T. Kariyado and Y. Hatsugai, Sci. Rep. **5**, 18107 (2015).

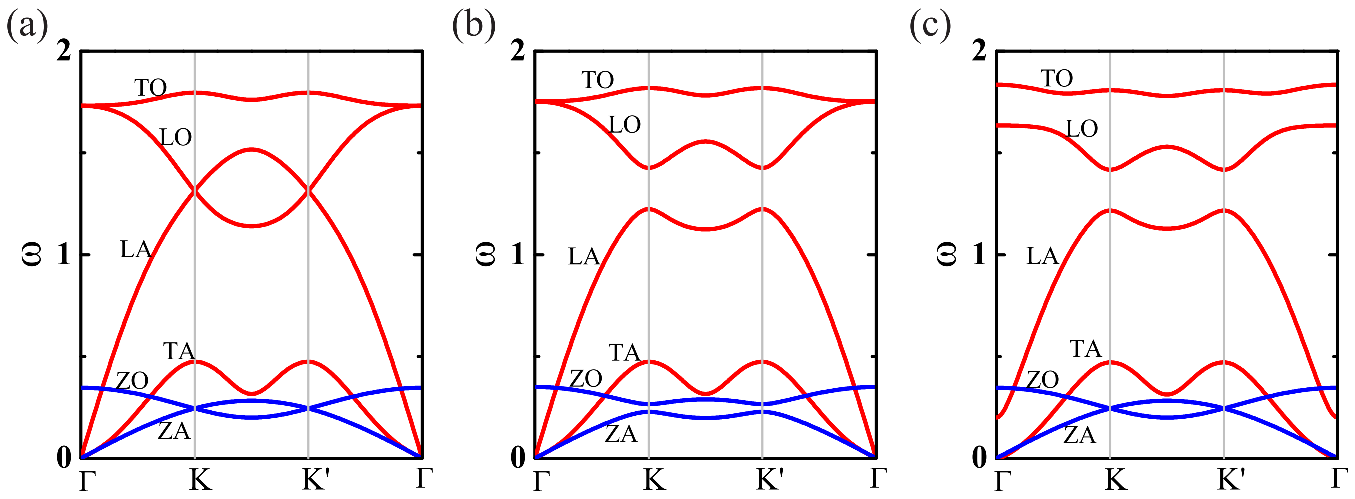


FIG. S2: (a-c) The Phonon dispersions same as Figs. 1(b-d), but including out-of-plane vibrations (blue lines, calcualted by using a force constant of 0.02 between the nearest neighbors).

[9] P. Wang, L. Lu, and K. Bertoldi, Phys. Rev. Lett. **115**, 104302 (2015).

[10] A. Maznev, A. Every, and O. Wright, Wave Motion **50**, 776 (2013).

[11] M. Büttiker, IBM J. Res. Dev. **32**, 63 (1988).

[12] S. Datta, Electronic transport in mesoscopic systems (Cambridge university press, 1997).
